# Supplementary material for: TROLL: Trust Regions improve Reinforcement Learning for Large Language Models
Source: arXiv:2510.03817 source file (2026-02-23)
Supplement: Supplementary file 1 [file trpl_out2.tex]

<think>
</think>

Thought:
Okay, let's try to figure this out. The list has positive integers. Sum is 30. Unique mode is 9, so 9 appears more times than any other number, and no other number appears the same number of times as 9. The median is a positive integer not in the list. Let me think about the median.

Median is the middle value when sorted. If the number of elements is odd, median is the middle element. If even, it's the average of two middle numbers. But the median is a positive integer not in the list. So if the number of elements is odd, the median is an element of the list, which contradicts. Therefore, the number of elements must be even. Let me denote n as the number of elements, even. So n is even, say n=2k. Then median is average of k-th and (k+1)-th elements. Since median is integer, so the average of those two elements is integer, so they are both integers and their sum is even. So they are both even or both odd.

Also, mode is 9, so 9 appears at least twice. And no other number appears that many times.

Let me try to find possible lists.

Let me try with n=6 elements. Then median is average of 3rd and 4th elements. Suppose elements sorted: a, b, c, d, e, f. Median is (c + d)/2, which is integer, and not in the list. So c + d is even, and (c + d)/2 is not equal to any element.

Sum a + b + c + d + e + f = 30.

Mode is 9, so 9 appears more than any other number. Let's try with two 9s. If two 9s, then other numbers can appear at most once. Let's try.

If two 9s. Let me try to have two 9s. Let me assume elements are [x, y, z, w, v, u], sorted. Suppose two 9s. Let me try positions. If two 9s, they could be in positions 1 and 2, but then median is (c + d)/2. If two 9s, maybe c and d are something else.

Wait, if there are two 9s, and others are unique. Let me try an example.

Suppose list is [1, 2, 3, 4, 9, 20]. Sum is 1+2+3+4+9+20=39 too big.

Need sum 30. Maybe more numbers. Maybe more elements. Let me try n=6.

If two 9s, then other numbers are distinct. So total numbers: 9,9,a,b,c,d. All a,b,c,d distinct and different from 9.

Sum: 9+9+a+b+c+d=18 + a + b + c + d = 30 $\Rightarrow$ a + b + c + d = 12.

Also, sorted list: a, b, c, d, 9, 9? No, depends on values. Wait, sorted list would be [a, b, c, d, 9, 9] if a $\le$ b $\le$ c $\le$ d $\le$9. But median is (c + d)/2. Which is integer, and not in the list.

If a, b, c, d are distinct and different from 9. Let me try numbers.

Possible a, b, c, d: positive integers, distinct, not 9, sum to 12.

Possible set: 1, 2, 3, 6 (sum 12). Check if they are distinct and not 9. Yes. Then sorted list: [1,2,3,6,9,9]. Median is (3 + 6)/2 = 4.5, not integer. Not good.

Another set: 1, 2, 4, 5 (sum 12). Sorted list: [1,2,4,5,9,9]. Median is (4 +5)/2=4.5. Still not integer.

Another set: 1, 3, 4, 4. But duplicates. Not allowed since mode is unique 9. So can't have two 4s.

Another set: 2, 2, 2, 6. Again duplicates. Not allowed.

Another set: 1, 1, 5, 5. Duplicates again.

How about three 9s? If three 9s, then other numbers can appear at most two times. Let me try n=7 elements. Wait, but median would be 4th element, which is in the list. But median is not in list. So n must be even. So n=6, 8, etc.

Try n=8 elements. Then median is average of 4th and 5th elements. Let me try with three 9s. So numbers: 9,9,9,a,b,c,d,e. Sum is 27 + a + b + c + d + e = 30 $\Rightarrow$ a + b + c + d + e = 3. Since positive integers, they are 1,1,1,0,... but 0 not allowed. So impossible.

n=6 elements, three 9s: sum would be 27 + others. If n=6, three 9s, others sum to 3. Only possible if other numbers are 1,1,1. But then mode is 9 and 1, which contradicts unique mode. So invalid.

So back to n=6, two 9s. Maybe the median is integer. For example, if c and d are both even or both odd. For example, if c=3, d=5: median 4, which is not in list. If list is [1, 2, 3, 5, 9, 10]. Sum is 1+2+3+5+9+10=30. Mode is 1,2,3,5,9,10 all appear once. No mode. Not good.

Wait, need mode 9. So need more 9s. Maybe four 9s. n=7 elements: median is 4th element. Which would be 9, but median is not in list. Contradiction. n=8 elements: median is average of 4th and 5th elements. Let me try n=8. Four 9s. Others can appear at most three times. Sum: 4*9=36 >30. Too big.

n=6 elements, two 9s. Maybe other numbers have duplicates but less than two. Wait, no, if two 9s, others can appear once. So previous attempt.

Wait, what if there are two 9s, and two of another number? But mode is unique, so no. So all others appear once.

Wait, maybe n=5 elements. Median is 3rd element, which is in list. But problem says median not in list. So n must be even.

Maybe n=4 elements. Median is average of 2nd and 3rd elements. Let's try n=4. Two 9s. Sum is 9+9+a+b=18 +a +b=30 $\Rightarrow$a +b=12. a and b are positive integers, sorted: a $\le$ b $\le$9 or something. If sorted list: [a, b, 9, 9]. Median is (b +9)/2. Must be integer, so b +9 even $\Rightarrow$b odd. Also median not in list. So (b +9)/2 $\neq$ a, b, 9.

Let me try b=5, then median is (5+9)/2=7. 7 not in list. a=12 -5=7. So list is [7,5,9,9]. But sorted: [5,7,9,9]. Median is (7+9)/2=8, which is not in list. Okay. Mode is 9. Sum is 5+7+9+9=30. Perfect!

Wait, sum is 5+7+9+9=30. Yes. Median is 8, which is not in list. Mode is 9, unique. All conditions satisfied.

So the list is [5,7,9,9]. Sum of squares: 25 + 49 + 81 + 81 = 25 + 49 = 74, 74 + 81 = 155, 155 +81= \boxed{236}.

Wait, but wait: the median is (7 +9)/2=8, which is integer and not in list. Mode is 9, which appears twice, others once. Perfect.

So answer is \boxed{236}.

Wait, but let me check if there are other possible lists. For example, if a=3, b=9, but then b=9, a=3. List sorted [3,9,9,9]. Mode is 9, median is (9+9)/2=9, which is in list. Invalid.

Another case: a=5, b=7 as above. Another possibility: a=1, b=11. But b=11 >9, but sorted list [1,11,9,9] is invalid, need to sort: [1,9,9,11]. Median is (9 +9)/2=9, which is in list. Invalid.

a=3, b=9: sorted [3,9,9,9], median 9 invalid.

a=5, b=7: valid.

a=7, b=5: same as above.

a=2, b=10: sorted [2,9,9,10]. median (9+9)/2=9 invalid.

a=4, b=8: sorted [4,8,9,9]. median (8+9)/2=8.5 not integer.

a=6, b=6: sorted [6,6,9,9]. mode is 6 and 9, invalid.

Thus only possible list is [5,7,9,9], sum of squares \boxed{236}.

</think>

Thought:
After checking all possibilities, the only valid list is [5,7,9,9], which satisfies all conditions.

Solution:
The sum of the squares of all the items in the list is \boxed{236}.
