# Supplementary material for: TROLL: Trust Regions improve Reinforcement Learning for Large Language Models
Source: arXiv:2510.03817 source file (2026-02-23)
Supplement: Supplementary file 2 [file vanilla_out2.tex]

<think>
</think>

Thought:
Okay, let's see. I need to find a list of positive integers where the sum is 30, the unique mode is 9, and the median is a positive integer that doesn't appear in the list. Then, I have to find the sum of the squares of all the items.

First, let's recall what each term means. The mode is the number that appears most frequently. Since it's the unique mode, 9 must appear more times than any other number. So, there has to be at least two 9s, and no other number can appear that many times.

The median is the middle number when the list is ordered. If the list has an odd number of elements, the median is the middle one. If even, it's the average of the two middle numbers. But the problem says the median is a positive integer that doesn't appear in the list. So, if the list has an even number of elements, the average of the two middle numbers must be an integer not in the list. If odd, the middle number must not be in the list. But since the median is a positive integer, and the list contains positive integers, that's possible.

Let me try to figure out the possible lengths of the list. Let's denote the length of the list as n.

If n is odd, say n = 2k + 1, then the median is the (k+1)th element. This median must not be in the list. But if the median is not in the list, then the (k+1)th element is some number not present in the list. But all elements are positive integers, so the median must be an integer. But how can the median not be in the list? For example, if the list is [1, 2, 3, 4, 5], the median is 3, which is in the list. But if the list is [1, 2, 4, 5], the median is (2+4)/2 = 3, which is not in the list. So, for even n, the median can be an integer not in the list.

So, maybe the list has an even number of elements. Let's assume that. Let's try n = 4. Then the median is the average of the second and third elements. Let's say the list is [a, b, c, d], sorted. Then median is (b + c)/2. This must be an integer not in the list.

But also, the sum is 30. And the mode is 9. So, 9 must appear at least twice. Let's try to construct such a list.

If n = 4, and mode is 9, then at least two 9s. Let's say two 9s. Then the other two numbers must be different from each other and from 9, or one of them could be same as another but not more than once. But since mode is unique, no other number can appear twice.

So, for example, [x, 9, 9, y], sorted. Then the median is (9 + 9)/2 = 9. But 9 is in the list, which violates the condition that the median is not in the list. So that's no good.

So, if we have two 9s, and the median is not 9, then the two middle numbers must not both be 9. So, maybe the list is [a, 9, 9, b], but sorted. If a and b are such that the median is not 9. But if a <= 9 <= b, then the median is (9 + 9)/2 = 9. So that's not possible. So, maybe we need more than two 9s?

If we have three 9s. Let's try n = 5. Then the median is the third element. If the list is [a, b, 9, c, d], sorted. Then the median is 9. But 9 is in the list, which violates the condition. So that's no good.

If n = 6. Then the median is the average of the third and fourth elements. Let's say the list is [a, b, x, y, c, d], sorted. Then median is (x + y)/2. This must be an integer not in the list.

Also, mode is 9. So, 9 must appear more times than any other number. Let's say 9 appears three times. Then other numbers can appear at most two times.

Let me try to construct such a list. Let's say the list has three 9s. Let's arrange them in the list. For example, [a, b, 9, 9, 9, d], sorted. Then the third and fourth elements are 9 and 9. So the median is (9 + 9)/2 = 9, which is in the list. Not allowed.

So, maybe the three 9s are not in the middle. Let's say the list is [a, 9, 9, 9, b, c], sorted. Then the third and fourth elements are 9 and 9. Again, median is 9. Not allowed.

So, maybe the three 9s are spread out. For example, [a, 9, b, 9, c, 9], sorted. Then the third and fourth elements are b and 9. So the median is (b + 9)/2. This must be an integer not in the list.

Let me pick b such that (b + 9) is even. So, b must be odd. Let's say b = 7. Then median is (7 + 9)/2 = 8. So 8 is the median, and it's not in the list. That works.

So, the list is [a, 9, 7, 9, c, 9], sorted. Wait, but sorted order would be [a, 7, 9, 9, c, 9]. But that's not sorted unless a <= 7 and c >= 9.

Let me make it sorted. Let's say a <= 7 <= 9 <= c <= 9. So, a <= 7, and c >= 9. But since there are three 9s, maybe c is 9. So the list is [a, 7, 9, 9, 9, 9]. But then the third and fourth elements are 9 and 9. Median is 9, which is in the list. Not allowed.

Hmm. So, maybe the three 9s are not consecutive. Let me try [a, 7, 9, 9, c, d], sorted. Then the third and fourth elements are 9 and 9. Median is 9. Not allowed.

So, maybe we need four 9s. Let's try that. If there are four 9s, then the mode is 9, and no other number appears more than three times.

Let's try n = 7. Then the median is the fourth element. If the list is [a, b, c, 9, d, e, f], sorted. Then the median is 9, which is in the list. Not allowed.

If n = 8. Then the median is the average of the fourth and fifth elements. Let's say the list is [a, b, c, x, y, z, w, v], sorted. Then median is (x + y)/2. This must be an integer not in the list.

If we have four 9s. Let's say the list is [a, b, c, 9, 9, 9, 9, d], sorted. Then the fourth and fifth elements are 9 and 9. Median is 9, which is in the list. Not allowed.

So, maybe the four 9s are spread out. For example, [a, b, 9, c, d, 9, e, 9], sorted. Then the fourth and fifth elements are c and d. So, median is (c + d)/2. Let's pick c and d such that this is an integer not in the list.

Let me try c = 7 and d = 9. Then median is (7 + 9)/2 = 8. Not in the list. So that works.

So the list is [a, b, 9, 7, 9, 9, e, 9], sorted. Wait, but sorted order would be [a, b, 7, 9, 9, 9, e, 9]. So, a and b must be <= 7, and e >= 9.

Let me pick a and b as small as possible. Let's say a = 1, b = 2. Then the list is [1, 2, 7, 9, 9, 9, e, 9]. Sorted, it would be [1, 2, 7, 9, 9, 9, e, 9]. But e must be >= 9. Let's say e = 9. Then the list is [1, 2, 7, 9, 9, 9, 9, 9]. But then the fourth and fifth elements are 9 and 9. Median is 9, which is in the list. Not allowed.

So, e must be greater than 9. Let's say e = 10. Then the list is [1, 2, 7, 9, 9, 9, 10, 9]. Sorted: [1, 2, 7, 9, 9, 9, 9, 10]. Now, the fourth and fifth elements are 9 and 9. Median is 9, which is in the list. Not allowed.

So, maybe c and d are not 7 and 9. Let's try c = 7 and d = 10. Then median is (7 + 10)/2 = 8.5, not an integer. Not allowed.

c = 6 and d = 10. Median is (6 + 10)/2 = 8. Good. So, the list is [a, b, 6, 9, 10, 9, e, 9], sorted. Wait, sorted would be [a, b, 6, 9, 9, 9, e, 10]. So, a and b <= 6, e >= 9.

Let me pick a = 1, b = 2. Then the list is [1, 2, 6, 9, 9, 9, e, 10]. Sorted: [1, 2, 6, 9, 9, 9, e, 10]. The fourth and fifth elements are 9 and 9. Median is 9, which is in the list. Not allowed.

So, maybe the fourth and fifth elements are not both 9. Let me try to have the four 9s spread out more. For example, [a, b, 9, c, d, 9, e, 9], sorted. Then the fourth and fifth elements are c and d. Let me pick c = 7 and d = 8. Then median is (7 + 8)/2 = 7.5, not integer.

c = 7 and d = 9. Median is 8. So, the list is [a, b, 9, 7, 9, 9, e, 9], sorted: [a, b, 7, 9, 9, 9, e, 9]. Again, fourth and fifth are 9 and 9. Median is 9.

This seems tricky. Maybe I need to have more than four 9s? Let's try five 9s.

If n = 9. Then the median is the fifth element. If the list is [a, b, c, d, 9, e, f, g, h], sorted. Then the median is 9, which is in the list. Not allowed.

If n = 10. Then the median is the average of the fifth and sixth elements. Let's say the list has five 9s. So, [a, b, c, d, 9, 9, 9, 9, 9, e], sorted. Then the fifth and sixth elements are 9 and 9. Median is 9, which is in the list. Not allowed.

So, maybe the five 9s are spread out. For example, [a, b, c, 9, d, e, f, 9, g, 9], sorted. Then the fifth and sixth elements are d and e. Let me pick d = 7 and e = 8. Then median is (7 + 8)/2 = 7.5, not integer.

d = 7 and e = 9. Median is (7 + 9)/2 = 8. Not in the list. So that works.

So the list is [a, b, c, 9, 7, 9, f, 9, g, 9], sorted. Wait, sorted would be [a, b, c, 7, 9, 9, f, 9, g, 9]. So, a, b, c <= 7, f >= 9, g >= 9.

Let me pick a = 1, b = 2, c = 3. Then the list is [1, 2, 3, 7, 9, 9, f, 9, g, 9]. Sorted: [1, 2, 3, 7, 9, 9, f, 9, g, 9]. The fifth and sixth elements are 9 and 9. Median is 9, which is in the list. Not allowed.

So, maybe the fifth and sixth elements are not both 9. Let me try to have the five 9s spread out more. For example, [a, b, 9, c, d, e, f, 9, g, 9], sorted. Then the fifth and sixth elements are d and e. Let me pick d = 7 and e = 8. Then median is (7 + 8)/2 = 7.5, not integer.

d = 7 and e = 9. Median is 8. So, the list is [a, b, 9, c, 7, 9, f, 9, g, 9], sorted: [a, b, 7, 9, 9, 9, f, 9, g, 9]. The fifth and sixth elements are 9 and 9. Median is 9.

This is really challenging. Maybe I need to go back to n = 6 and try again.

Let me try n = 6, with three 9s. The median is (third + fourth)/2. Let me have the list [a, b, 7, 9, c, d], sorted. Then the third and fourth elements are 7 and 9. Median is (7 + 9)/2 = 8. Not in the list. That works!

So, the list is [a, b, 7, 9, c, d], sorted. With three 9s. So, one of a, b, c, d is 9. Let's say c and d are 9. So, the list is [a, b, 7, 9, 9, 9], sorted. Then a and b <= 7.

Let me pick a = 1, b = 2. Then the list is [1, 2, 7, 9, 9, 9]. Sum is 1 + 2 + 7 + 9 + 9 + 9 = 37. Too much.

We need sum to be 30. So, let's adjust. Let me try a = 1, b = 1. Then the list is [1, 1, 7, 9, 9, 9]. Sum is 1 + 1 + 7 + 9 + 9 + 9 = 36. Still too much.

a = 1, b = 2, and change 7 to something smaller. But 7 is the third element. If I make it 6, then the list is [1, 2, 6, 9, 9, 9]. Sum is 1 + 2 + 6 + 9 + 9 + 9 = 36. Still too much.

Maybe a = 1, b = 1, and third element is 5. Then list is [1, 1, 5, 9, 9, 9]. Sum is 1 + 1 + 5 + 9 + 9 + 9 = 34. Still too much.

a = 1, b = 1, third = 4. Sum is 1 + 1 + 4 + 9 + 9 + 9 = 33.

a = 1, b = 1, third = 3. Sum is 1 + 1 + 3 + 9 + 9 + 9 = 32.

a = 1, b = 1, third = 2. Sum is 1 + 1 + 2 + 9 + 9 + 9 = 31.

a = 1, b = 1, third = 1. Sum is 1 + 1 + 1 + 9 + 9 + 9 = 30. Perfect!

So the list is [1, 1, 1, 9, 9, 9]. Sorted. Let's check the conditions:

- Sum is 1 + 1 + 1 + 9 + 9 + 9 = 30. Check.
- Mode is 9, which appears three times. Other numbers appear once or twice. So unique mode is 9. Check.
- Median is (third + fourth)/2 = (1 + 9)/2 = 10/2 = 5. 5 is not in the list. Check.

So this list satisfies all conditions!

Now, the sum of the squares is 1${}^2$ + 1${}^2$ + 1${}^2$ + 9${}^2$ + 9${}^2$ + 9${}^2$ = 1 + 1 + 1 + 81 + 81 + 81 = 3 + 243 = 246.

So the answer is \boxed{246}.

But wait, let me check if there are other possible lists. For example, could there be a list with more elements?

But given the constraints, this seems to be the only possible list. So I think
